# Supplementary material for: Calculation of phase diagrams in the multithermal-multibaric ensemble
Source: arXiv:1904.05624 ancillary file (2019-06-04)
Supplement: Supplementary file 1 [file SupplementaryInformation.pdf]

# Supplementary information to: Phase diagrams from single molecular dynamics simulations

**Pablo M. Piaggi and Michele Parrinello**
Department of Chemistry and Applied Biosciences, ETH Zurich, c/o USI Campus, Via Giuseppe Buffi 13, CH-6900, Lugano, Switzerland
Facoltà di Informatica, Istituto di Scienze Computazionali, and National Center for Computational Design and Discovery of Novel Materials (MARVEL), Università della Svizzera italiana (USI), Via Giuseppe Buffi 13, CH-6900, Lugano, Switzerland
e-mail: parrinello@phys.chem.ethz.ch

April 23, 2019

## Sodium

In Fig. SI-1 we show the trajectories of the multithermal-multibaric and isothermal-isobaric simulations of sodium. The fluctuations of the energy and the volume are much larger in the multithermal-multibaric ensemble. In both ensembles $s$ is sampled from 0 to the total number of atoms (250). This shows the efficient and reversible transformation between the liquid and the bcc phase. This is crucial to obtain converged estimates of the free energy differences.

The increase in the fluctuactions of energy and volume is also shown in Fig. SI-2 where the energy vs the volume is plotted. The region sampled in the multithermal-multibaric case is much larger than in the isothermal-isobaric ensemble. The exact region that is sampled in the multithermal-multibaric ensemble is determined by the condition that configurations relevant at all chosen temperatures and pressures must be sampled in the simulation. The points have been divided into two groups, those pertaining to the liquid ($s < 125$) and those that are consistent with solid configurations ($s > 125$).

## Aluminum

As in the case of sodium we show the constriction of the configuration space in the dimension of the order parameter. To this end we plotted contour surfaces of the free enery as a function of the energy, the volume and the order parameter for the fcc and bcc case. These are shown in Fig. SI-3. These surfaces are also shaped as an hourglass and show the bottleneck in the order parameter dimension.

We also plot the energy, volume and order parameter vs. time in Figs. SI-4 and SI-6, and the energy vs. volume in Figs. SI-5 and SI-7.

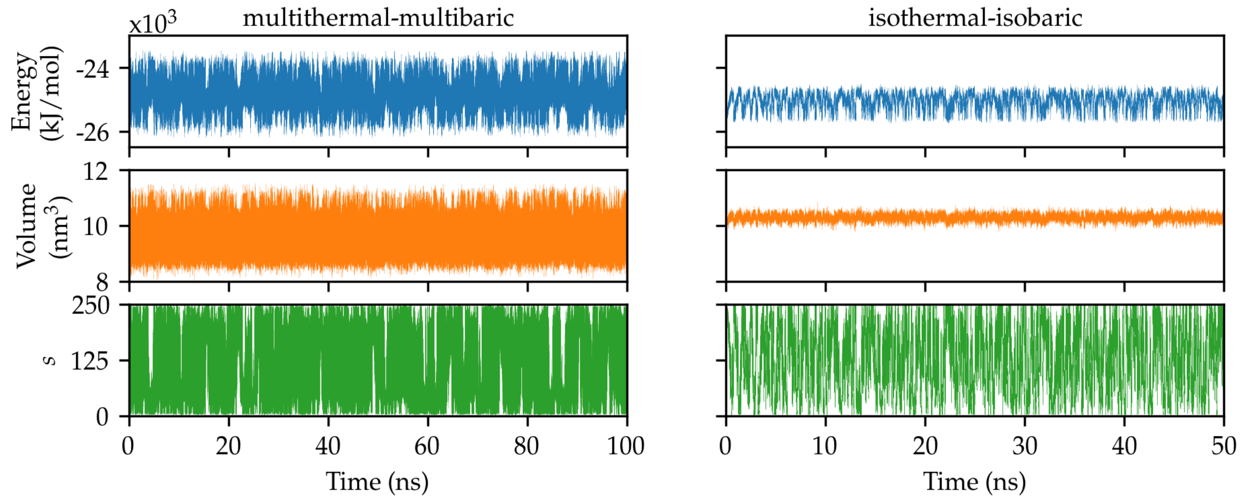


**Fig. SI-1 | Energy, volume and order parameter $s$ vs. time for the simulations of sodium.** Left) Multithermal-multibaric simulation spanning the temperature range 350-450 K and the pressure range 0-1 GPa. Right) Isothermal-isobaric simulation at 375 K and 1 bar. As expected, the amplitude of the fluctuations of the energy and volume are much larger in the multithermal-multibaric ensemble.

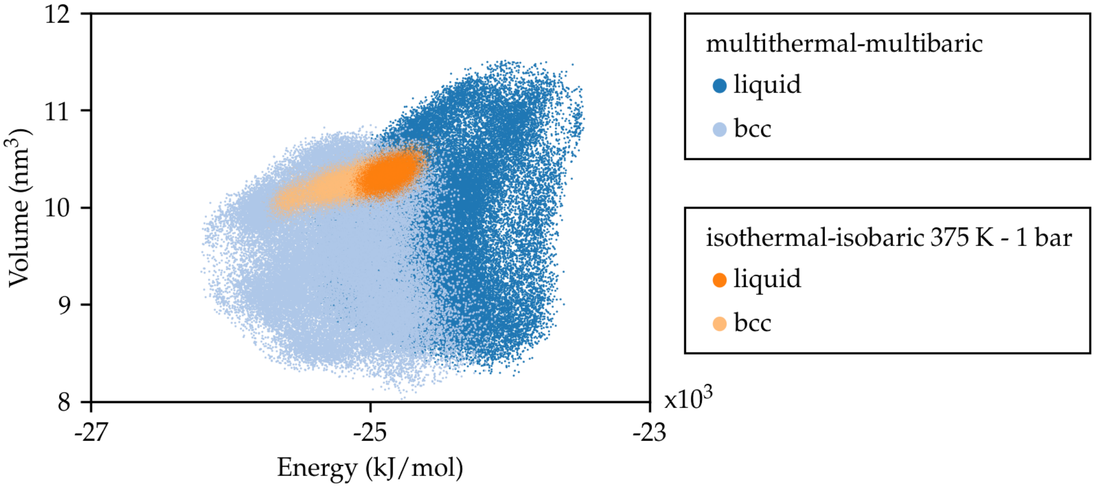


**Fig. SI-2 | Energy vs. volume for the simulations of sodium.** The region explored in the multithermal-multibaric ensemble is much larger than in the isothermal-isobaric ensemble.

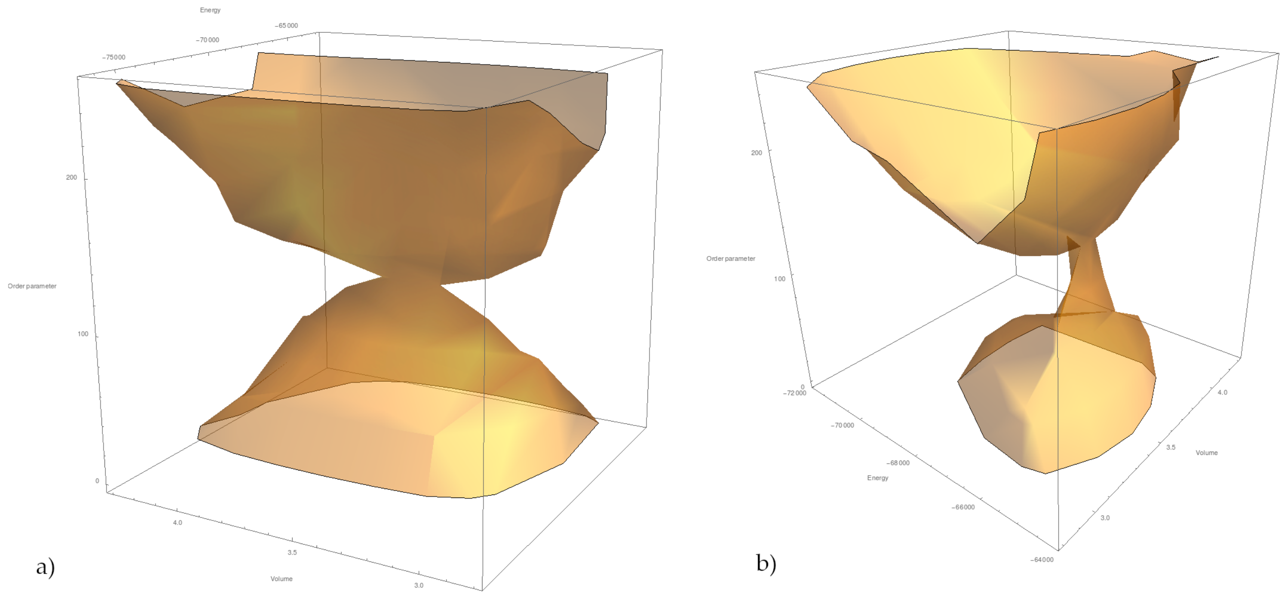


**Fig. SI-3 | Free energy contour surfaces for aluminum.** The free energies are functions of the energy, the volume, and the order parameter $s$. a) fcc-liquid free energy contour surface and b) bcc-liquid free energy contour surface. Both surfaces show constriction in the dimension of the order parameter.

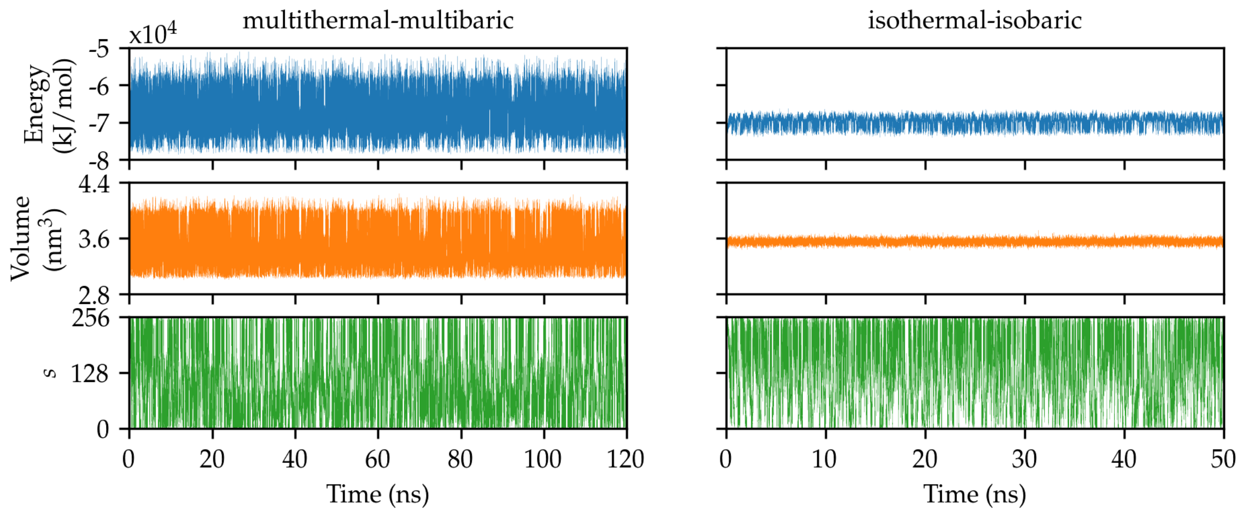


**Fig. SI-4 | Energy, volume and order parameter** $s$ **vs. time for the simulations of fcc aluminum.** Left) Multithermal-multibaric simulation spanning the temperature range 1800-2400 K and the pressure range 20-40 GPa. Right) Isothermal-isobaric simulation at 2000 K and 30 GPa.

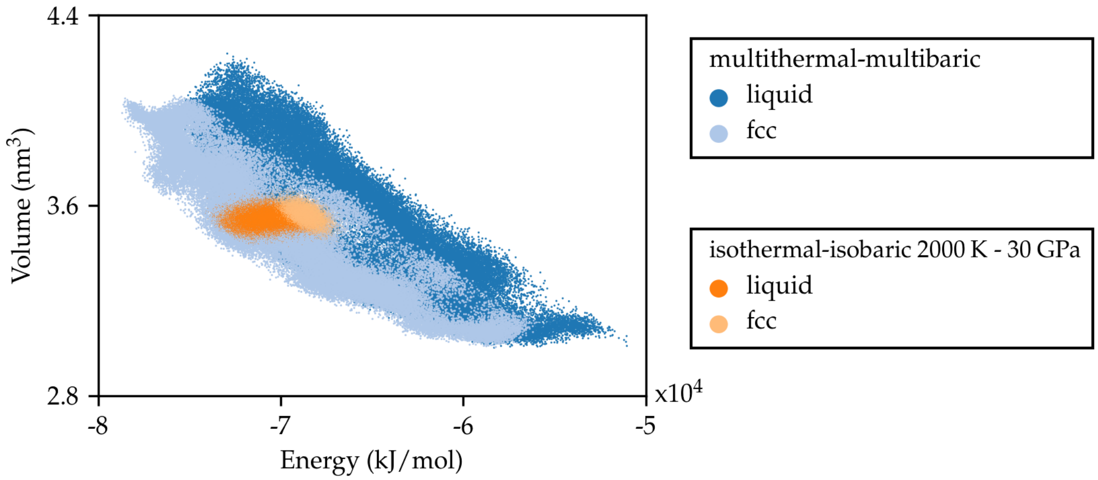


**Fig. SI-5 | Energy vs. volume for the simulations of fcc aluminum.**

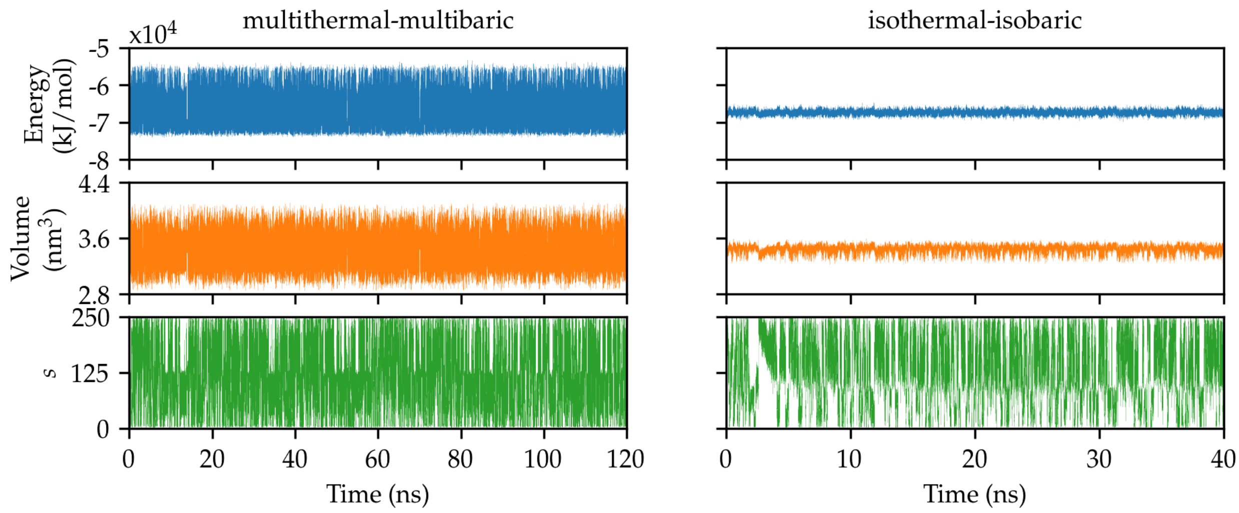


**Fig. SI-6 | Energy, volume and order parameter $s$ vs. time for the simulations of bcc aluminum.** Left) Multithermal-multibaric simulation spanning the temperature range 1800-2400 K and the pressure range 20-40 GPa. Right) Isothermal-isobaric simulation at 2000 K and 30 GPa.

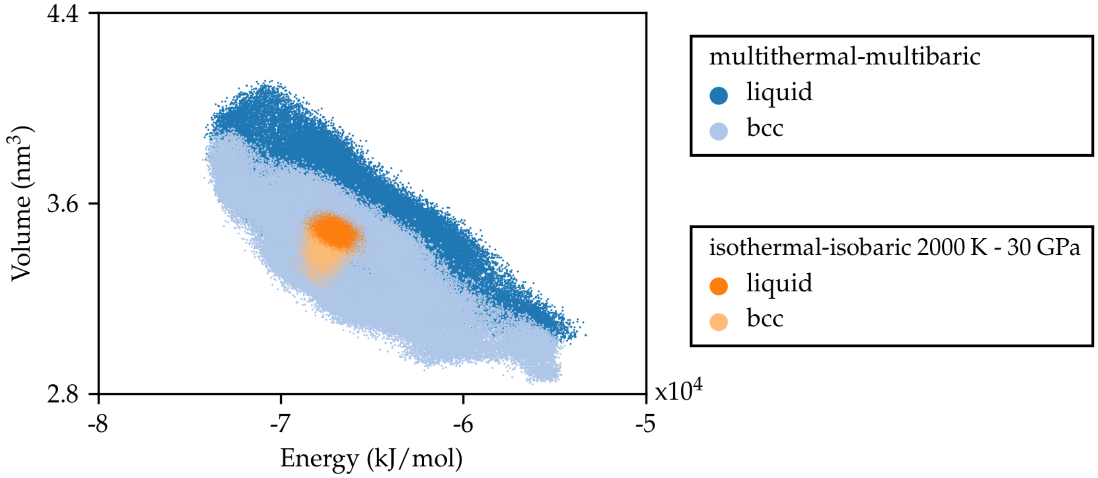


**Fig. SI-7 | Energy vs. volume for the simulations of bcc aluminum.**
